# Supplementary material for: Evidence for modification of $b$ quark hadronization in high-multiplicity $pp$ collisions at $\sqrt{s} = 13$ TeV
Source: arXiv:2204.13042 source file (2023-10-13)
Supplement: Supplementary file 1 [file supplementary.tex]

\clearpage
\FloatBarrier
\section*{Appendix: Supplemental material}
\label{sec:Supplementary}  

The ratio of $\Bs$ to $\Bd$ cross-sections $\sigma_{\Bs}/\sigma_{\Bd}$ versus the number of VELO tracks and number of backward VELO tracks are given in Table \ref{tab:tab1} and Table \ref{tab:tab2}, respectively, for the transverse momentum range range $0<\pt<20 \gevc$.  Tables \ref{tab:tab3}, \ref{tab:tab4}, and \ref{tab:tab5} give the ratio versus the number of VELO tracks over the transverse momentum ranges $0<\pt<6 \gevc$, $6<\pt<12 \gevc$, and $12<\pt<20 \gevc$, respectively.

\begin{table}[h]
\centering
\begin{tabular}{cccc}
$\Nvelo$ & $\sigma_{\Bs}/\sigma_{\Bd}$ &Uncorrelated uncertainty&Correlated uncertainty\\
\midrule
5-20  & 0.23 & 0.06 & 0.02 \\
21-30 & 0.29 & 0.05 & 0.03 \\
31-40 & 0.24 & 0.03 & 0.02 \\
41-50 & 0.27 & 0.03 & 0.02 \\
51-60 & 0.29 & 0.03 & 0.03 \\
61-70 & 0.29 & 0.03 & 0.03 \\
71-80 & 0.32 & 0.03 & 0.03 \\
81-100 & 0.31 & 0.03 & 0.03 \\
101-125 & 0.33 & 0.03 & 0.03 \\
126-150 & 0.36 & 0.06 & 0.03 \\
151-250 & 0.35 & 0.10 & 0.03 \\
\end{tabular}
\caption{Ratio of cross-sections $\sigma_{\Bs}/\sigma_{\Bd}$ in the range $0<\pt<20 \gevc$ versus $\Nvelo$. }
\label{tab:tab1}
\end{table}

\begin{table}[!htb]
\centering
\begin{tabular}{cccc}
$\Nback$ & $\sigma_{\Bs}/\sigma_{\Bd}$ &Uncorrelated uncertainty&Correlated uncertainty\\
\midrule
1-10 & 0.27 & 0.02 & 0.02 \\
11-15 & 0.29 & 0.02 & 0.03 \\
16-20 & 0.33 & 0.03 & 0.03 \\
21-25 & 0.29 & 0.03 & 0.03 \\
26-30 & 0.29 & 0.03 & 0.03 \\
31-40 & 0.32 & 0.03 & 0.03 \\
41-60 & 0.30 & 0.04 & 0.03 \\
\end{tabular} 
\caption{Ratio of cross-sections $\sigma_{\Bs}/\sigma_{\Bd}$ in the range $0<\pt<20 \gevc$ versus $\Nback$. }
\label{tab:tab2}
\end{table}

\begin{table}
\centering
\begin{tabular}{cccc}
$\Nvelo$ & $\sigma_{\Bs}/\sigma_{\Bd}$ &Uncorrelated uncertainty&Correlated uncertainty\\
\midrule
5-20 & 0.18 & 0.06 & 0.02 \\
21-30 & 0.27 & 0.06 & 0.02 \\ 
31-40 & 0.24 & 0.04 & 0.02 \\
41-50 & 0.24 & 0.04 & 0.02 \\
51-60 & 0.31 & 0.05 & 0.03 \\ 
61-70 & 0.29 & 0.05 & 0.03 \\
71-80 & 0.45 & 0.09 & 0.04 \\
81-100 & 0.35 & 0.05 & 0.03 \\
101-125 & 0.38 & 0.07 & 0.03 \\
126-150 & 0.45 & 0.15 & 0.04 \\
151-250 & 0.47 & 0.31 & 0.04 \\
\end{tabular}
\caption{Ratio of cross-sections $\sigma_{\Bs}/\sigma_{\Bd}$ in the range $0<\pt<6 \gevc$ versus $\Nvelo$. }
\label{tab:tab3}
\end{table}

\begin{table}
\centering
\begin{tabular}{cccc}
$\Nvelo$ & $\sigma_{\Bs}/\sigma_{\Bd}$ &Uncorrelated uncertainty&Correlated uncertainty\\
\midrule
5-20 & 0.26 & 0.11 & 0.02 \\
21-30 & 0.28 & 0.07 & 0.02 \\
31-40 & 0.25 & 0.04 & 0.02 \\
41-50 & 0.33 & 0.05 & 0.03 \\
51-60 & 0.27 & 0.04 & 0.02 \\
61-70 & 0.35 & 0.05 & 0.03 \\
71-80 & 0.25 & 0.03 & 0.02 \\
81-90 & 0.28 & 0.03 & 0.02 \\
101-125 & 0.30 & 0.04 & 0.03 \\
126-150 & 0.34 & 0.07 & 0.03 \\
151-250 & 0.20 & 0.08 & 0.02 \\
\end{tabular} 
\caption{Ratio of cross-sections $\sigma_{\Bs}/\sigma_{\Bd}$ in the range $6<\pt<12 \gevc$ versus $\Nvelo$. }
\label{tab:tab4}
\end{table}

\begin{table}
\centering
\begin{tabular}{cccc}
$\Nvelo$ & $\sigma_{\Bs}/\sigma_{\Bd}$ &Uncorrelated uncertainty&Correlated uncertainty\\
\midrule
5-30 & 0.40 & 0.23 & 0.04 \\
31-50 & 0.20 & 0.04 & 0.02 \\
51-70 & 0.20 & 0.03 & 0.02 \\
71-90 & 0.31 & 0.06 & 0.03 \\
91-125 & 0.27 & 0.06 & 0.03 \\
126-250 & 0.30 & 0.11 & 0.03 \\
\end{tabular} 
\caption{Ratio of cross-sections $\sigma_{\Bs}/\sigma_{\Bd}$ in the range $12<\pt<20 \gevc$ versus $\Nvelo$. }
\label{tab:tab5}
\end{table}

\FloatBarrier
